# Supplementary material for: Characterizing gas flow from aerosol particle injectors
Source: arXiv:1609.09020 source file (2017-04-18)
Supplement: Supplementary file 1 [file PlasmaImaging_SI.pdf]

# Supplementary Information:
# Characterizing gas flow from aerosol particle injectors

Daniel A. Horke,[1,2,*] Nils Roth,[1,3] Lena Worbs,[1] and Jochen Küpper[1,2,3]

[1] *Center for Free-Electron Laser Science, DESY, Notkestrasse 85, 22607 Hamburg, Germany*
[2] *The Hamburg Center for Ultrafast Imaging, University of Hamburg, Luruper Chaussee 149, 22761 Hamburg, Germany*
[3] *Department of Physics, University of Hamburg, Luruper Chaussee 149, 22761 Hamburg, Germany*
(Dated: January 31, 2017)

## I. PRESSURE CALIBRATION

For calibration of the observed plasma-glow intensity in the image against a known density of helium gas, the injector tip and mounting was removed from the chamber and the entire chamber flooded with helium gas at known, constant pressures in the range from 0.8 to 4.1 mbar, measured by the capacitive gauge. During these measurements the turbomolecular pump is switched off and the chamber is pumped by the roughing pump, ensuring a constant replenishment of the helium. An example image of a produced plasma is shown in the inset of Figure S1.

To calibrate the recorded image intensity with respect to the chamber pressure, we record 20 images at a given pressure, and repeat this for different camera exposure times, each chosen such that no saturation occurs and the plasma is clearly visible. All other camera settings are kept constant during all measurements. A dark image (laser off) is taken for each exposure time and substracted from the measurements. We then take the average of the background-corrected frames at a fixed exposure time and scale the intensity accordingly by dividing every pixel intensity by the known exposure time, increasing the effective dynamic range of our measurements. For calibration purposes we only consider the brightest central region of the produced plasma and take the average intensity of those brightest $100 \times 50$ pixels. The resulting calibration curve, i. e., the average intensity per pixel per millisecond exposure time ($I$/pix/ms) as a function of pressure, is shown in Figure S1. These calibration measurements are fit to a power law $I = A \times P^x + c$, shown as red line in Figure S1, to produce a continuous colorscale for subsequent measurements. Furthermore, the

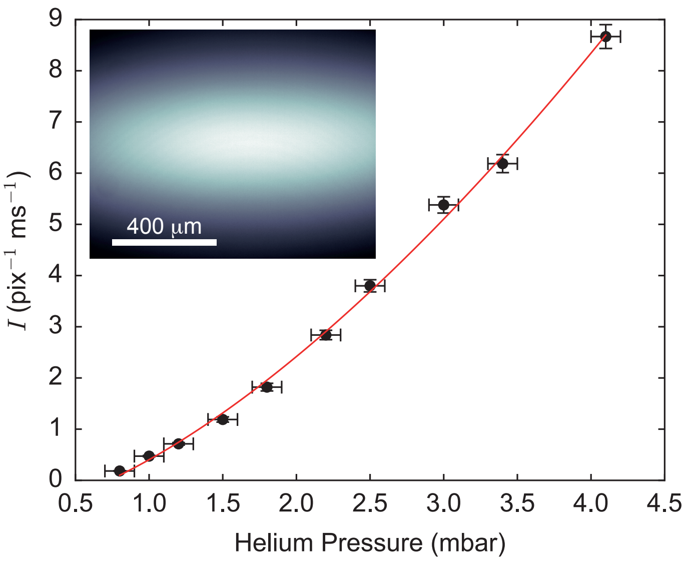


FIG. S1. Calibration curve showing the the average intensity per pixel per millisecond exposure time of the most intense region of the plasma as a function of chamber pressure. The red line indicates a power law fit used to create a continuous pressure scale. Shown inset is an background subtracted image showing the plasma produced at 4.1 mbar of helium.

* daniel.horke@cfel.de;
https://www.controlled-molecule-imaging.org

measured helium pressures can be converted into number densities; assuming ideal-gas behavior and room temperature, 1 mbar corresponds to $2.4 \times 10^{16}$ cm$^{-3}$.

## II. SPATIAL PRESSURE PROFILES

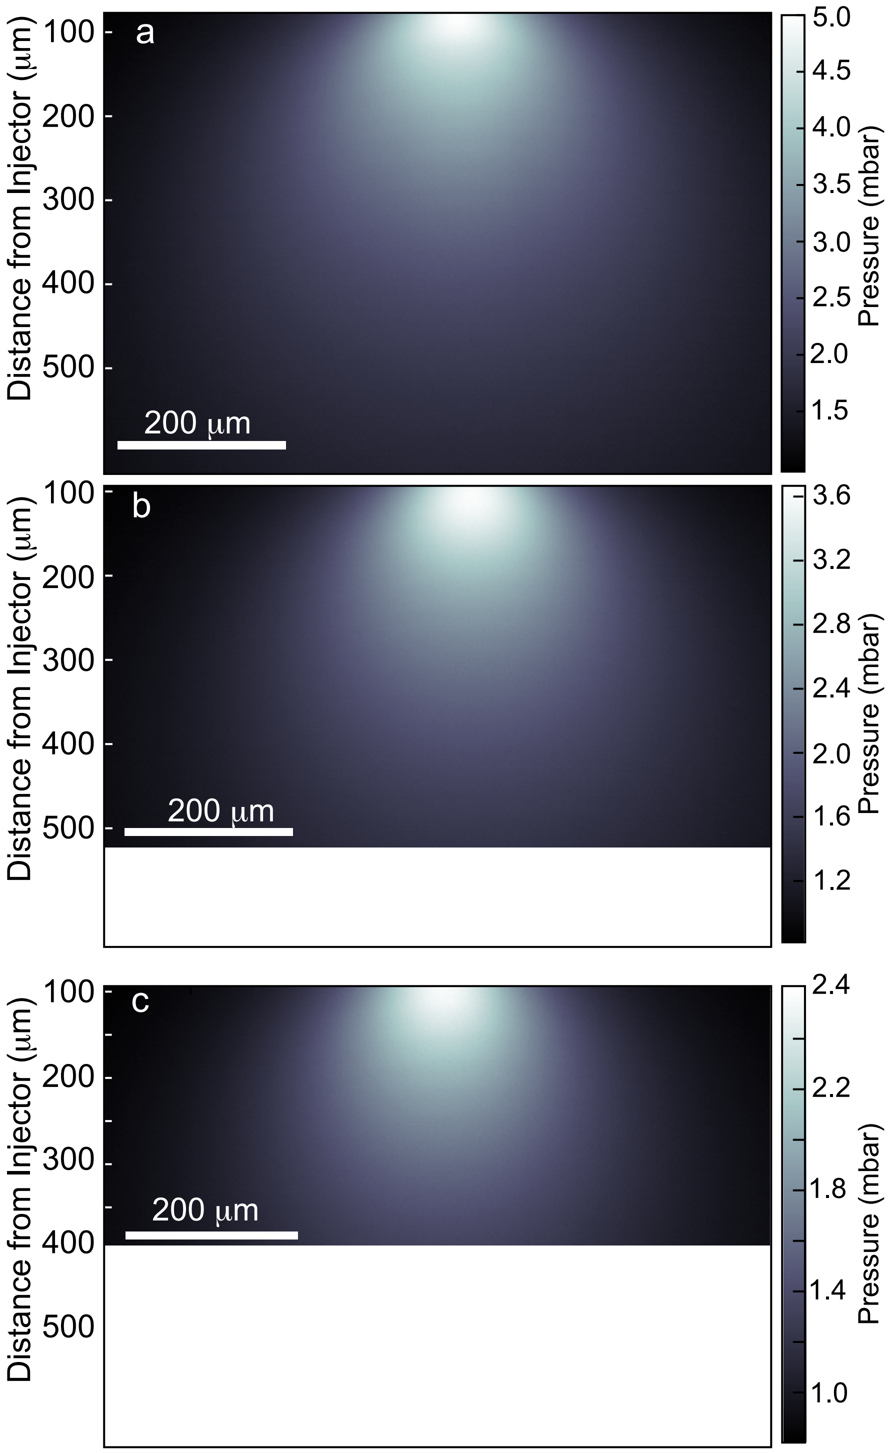


FIG. S2. Spatial distribution of gas-flow from the injector tip with a) 800 mbar, b) 500 mbar, and c) 300 mbar upstream pressure; note the distinct intensity scales.

## III. RADIAL GAS DENSITY PROFILES

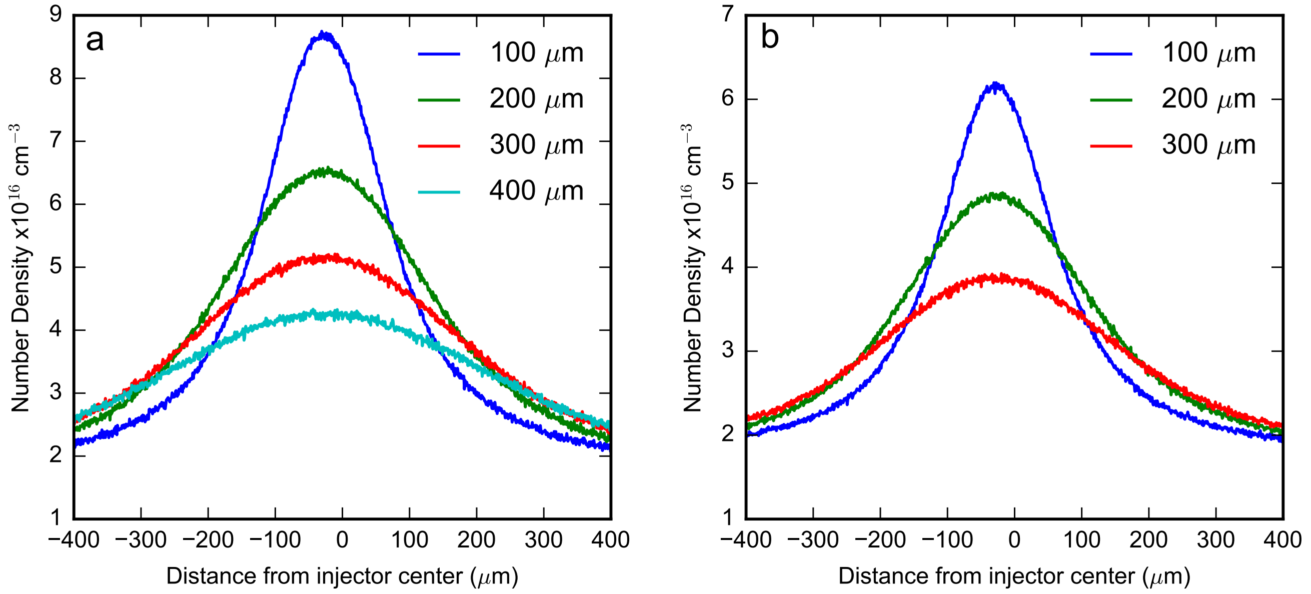


FIG. S3. Radial pressure distribution at specified heights below the injector tip for a) 500 mbar and b) 300 mbar upstream pressure.
